# Supplementary material for: SmartAvatar: Text- and Image-Guided Human Avatar Generation with VLM AI Agents
Source: arXiv:2506.04606 source file (2025-06-05)
Supplement: Supplementary file 1 [file appendix.tex]

\section{Appendix (Informal)}

\subsection{User Customization}
\begin{figure}
    \centering
    \includegraphics[width=0.75\linewidth]{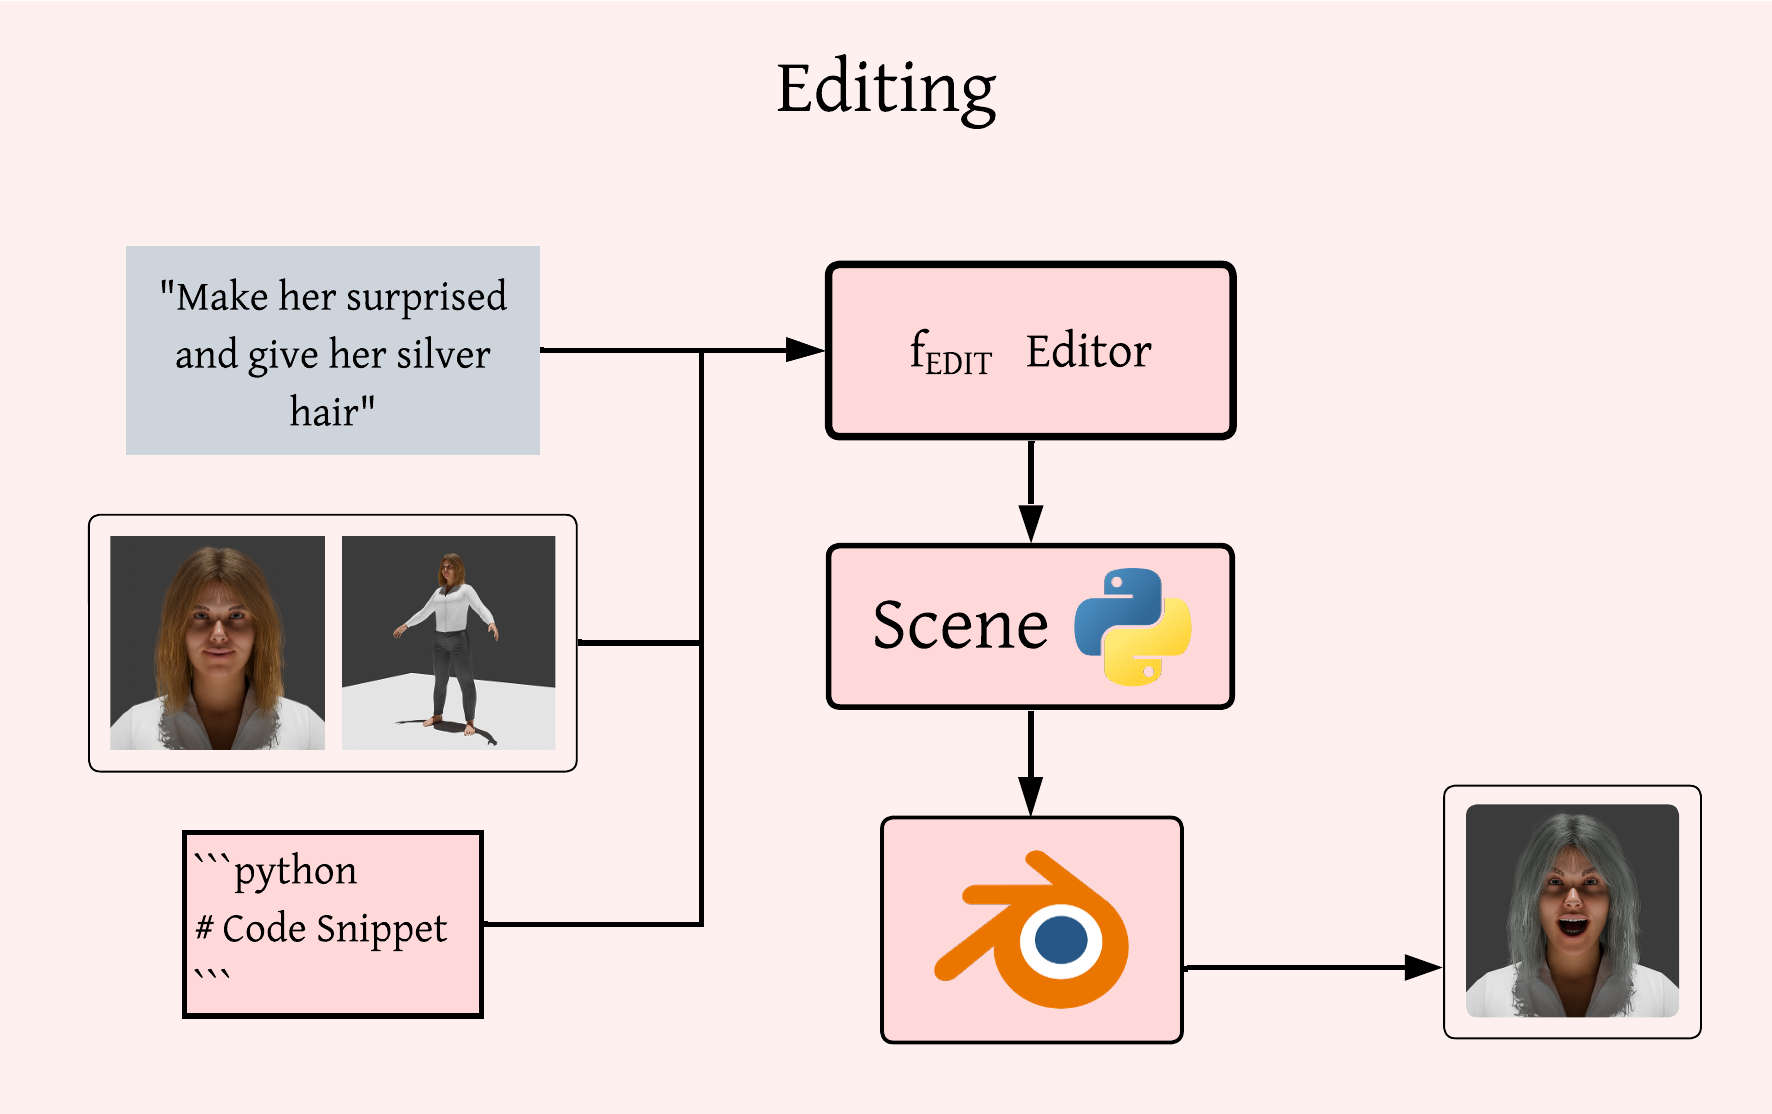}
    \caption{SmartAvatar pipeline: (1) Descriptor LLM extracts semantic attributes; (2) Generator LLM creates Blender Python code; (3) Refiner LLM optionally adjusts code based on visual feedback; (4) final avatar is rendered when similarity exceeds a threshold or max iterations are reached.
    Editing pipeline: the Editor LLM takes the rendered avatar, associated code snippet, and editing instructions, along with detailed CoT prompts. It first reasons about which features are relevant to the edit instructions and then determines how to best modify the code to fit the desired output. \textcolor{red}{Let's move this figure to supplementary materials.}}
    \label{fig:editing}
\end{figure}

\subsubsection{Descriptor}
\begin{shaded}
    "Analyze the following photo and describe the person's appearance for 3D model generation: 
    Include general features such as age, appearance, and any general traits, in addition to finer grained facial details."
\end{shaded}
\subsubsection{Generator}
\begin{shaded}
    "Based on this description for 3D model creation:
            <description>
            Provide only the Python snippet bounded by '\# region RENDER\_SNIPPET'  and '\# endregion'
            that sets up the model accordingly.
            Then check that snippet with Python's built-in compiler
            (e.g. 'python -m py\_compile'); correct any syntax errors before you output."
\end{shaded}
\subsubsection{Refiner}
\begin{shaded}
    inputs = [
        \# A) The full reference of valid presets \& keys
        {"type": "input\_text",  "text": options\_md},

        \# B) Reference photo
        {"type": "input\_text",  "text": "Here is the reference photo:"},
        {"type": "input\_image", "image\_url": f"data:image/jpeg;base64,{b64\_o}"},

        \# C) Current render
        {"type": "input\_text",  "text": "Here is the rendered portrait based on this code:"},
        {"type": "input\_image", "image\_url": f"data:image/jpeg;base64,{b64\_p}"},

        \# D) The snippet to refine
        {"type": "input\_text",  "text": f"```python\\n{current\_snippet}\\n```"},

        \# E) Stronger, explicit chain‑of‑thought + inline comments
        {
            "type": "input\_text",
            "text": f"""Iteration {iteration} - follow these three phases exactly:

\#\#\# 1. ANALYSIS PHASE (one sentence per category)
Go in this order and for each category write exactly one bullet identifying any mismatch:
- **Preset** (e.g. ethnicity/face shape preset)
- **Skin** (tone \& texture)
- **Hair** (quality, shader, style, color)
- **Eyes** (shape, color)
- **Age \& Height**
- **Body proportions**
- **Facial proportions** (nose, brows, cheeks, mouth, chin, jaw, ears)

\#\#\# 2. EDIT PHASE (code + inline comments)
For each bullet above, immediately propose the exact code change. Use inline Python comments (\# …) to tag which feature you're addressing, e.g.:

```python
\# region RENDER\_SNIPPET
\# Initialize with a preset
my\_human = Human.from\_preset(r"models/male/Asian presets/Asian 3.json")

\# Hair colour too warm - reduce redness
my\_human.hair.regular\_hair.redness = -0.3
```
Always preserve unchanged variables by re-emitting their previous values. Remember to preserve unchanged presets with the previous preset loading.

\#\#\# 3. OUTPUT PHASE
- Wrap only your edited snippet between:
```python
\# region RENDER\_SNIPPET
...your code with inline comments...
\# endregion
```

- At the very top of that region, include a short 3-5 bullet summary of your Analysis Phase, each prefixed \# ANALYSIS:.
- If no edits are needed ($\geq$90\% accurate), output exactly:
```
\# NO\_CHANGES
```
\#\#\# REMEMBER TO INITIALIZE THE HUMAN OBJECT WITH A PRESET `my\_human = Human.from\_preset(...)`
\#\#\# DO NOT CHANGE THE PRESET UNLESS IT IS INCORRECT. IT IS CRUCIAL TO START WITH A PRESET.
"""
        }
    ]
\end{shaded}
